# Supplementary material for: One-step Targeted Maximum Likelihood for Time-to-event Outcomes
Source: arXiv:1802.09479 source file (2019-06-12)
Supplement: Supplementary file 1 [file appendix.tex]

\section*{Appendix}
\label{sec:appendix}

\subsection{Proof that our proposed submodel (\ref{eq:1dULFM}) is a universal least favorable submodel}
Clearly, it is a submodel so that for each $\varepsilon$ it yields a hazard, and
that it contains $\lambda _{0,N}$ at $\varepsilon= 0$. Recall the loss function
(\ref{eq:likeli}) evaluated at $\lambda _{n,N}^{ULFM}(\varepsilon)$:
\begin{align*}
\mathcal{L}(p_\varepsilon) &=  - \log p(\lambda _{n,N}^{ULFM}(\varepsilon))\\
&\propto - \sum_{t \leqslant k} {\{dN(t)\log \lambda
_{n,N}^{ULFM}(\varepsilon)(t|A,W) + (1 - dN(t))\log (1 - \lambda
_{n,N}^{ULFM}(\varepsilon)(t|A,W))\}}
\end{align*}
Use the property of (\ref{eq:1dULFM}) we have
\begin{align*}
\frac{\partial}{\partial\varepsilon}\{ {dN(t)\log \lambda
_{0,N}^{ULFM}(\varepsilon)(t|A,W) + ( {1 - dN(t)} )\log ( {1 - \lambda
_{0,N}^{ULFM}(\varepsilon)(t|A,W)} )} \} \\
= - h_{d,k}(g_{0,A},\bar S_{0,A_c},{S_{0,N}^{ULFM}(\varepsilon)})[ {dN(t) -
{\lambda _{0,N}^{ULFM}}(\varepsilon )(t|A,W)} ]
\end{align*}
Plug into the loss function, we have the score of $\mathcal{L}(\lambda _{n,N}^{ULFM}(\varepsilon )) ( O ) $ at $\varepsilon$ is given by
\begin{align*}
\frac{\partial}{\partial\varepsilon} \mathcal{L}({\lambda
_{n,N}^{ULFM}(\varepsilon))(O)} & = \sum_{t \leqslant k} {h_{d,k}(g_{0,A},{\bar
G_{0,A_c}},{S_{0,N}^{ULFM}(\varepsilon)})[ {dN(t) - {\lambda
_{0,N}^{ULFM}(\varepsilon)}(t|A,W)} ]}\\
& = \sum_t {h_{d,k}}( {g_{0,A},{\bar G_{0,A_c}},{S_{0,N}^{ULFM}(\varepsilon)}}
)\biggl[ I( {\widetilde T = t,\Delta  = 1} )\\
& - I(\widetilde T \geqslant t)\lambda _{0,N}^{ULFM}(\varepsilon)(t|A
= d(W),W) \biggr]\\
& = D^*_{1,d,k}(g_{0,A},\bar G_{0,A_c},S_{0,N}^{ULFM}(\varepsilon)),
\end{align*}
explicitly proving that indeed this is a universal least favorable model for $
\lambda_{n,N}$.
